# Supplementary material for: Zerrow: True Zero-Copy Arrow Pipelines in Bauplan
Source: arXiv:2504.06151 source file (2025-05-13)
Supplement: Supplementary file 1 [file appendix.tex]

\appendix
\section{Appendix}
